# Supplementary material for: Relativistic acceleration of electrons injected by a plasma mirror into a radially polarized laser beam
Source: arXiv:2004.03979 source file (2020-04-08)
Supplement: Supplementary file 1 [file SupplementalMaterial.pdf]

# Supplemental material for: Relativistic acceleration of electrons injected by a plasma mirror into a radially polarized laser beam -

N. Zaïm, M. Thévenet, A. Lifschitz, J. Faure

*LOA, ENSTA ParisTech, CNRS, Ecole polytechnique,*

*Université Paris-Saclay, 828 bd des Maréchaux, 91762 Palaiseau cedex France*

## MODELING FEW-CYCLE AND TIGHTLY FOCUSED RADIALLY POLARIZED LASER PULSES

We use an exact analytical solution of Maxwell's equations to model an ultrashort non-paraxial radially polarized laser beam. The expression of the field is obtained by using the complex source/sink model to find the Hertz potential of the pulsed beam. [1] A Poisson-like spectrum is used to correctly describe the few-cycle pulse. [1, 2] The obtained fields correspond to the real part of these expressions, in cylindrical coordinates:

$$E_z(\mathbf{r},t) = \frac{A_0}{\widetilde{R}}\left[\frac{3\cos^2\widetilde{\Theta}-1}{\widetilde{R}}\left(\frac{G_-^{(0)}}{\widetilde{R}}+\frac{G_+^{(1)}}{c}\right)-\frac{\sin^2\widetilde{\Theta}}{c^2}G_-^{(2)}\right] \tag{1}$$

$$E_r(\mathbf{r},t) = \frac{3A_0\sin 2\widetilde{\Theta}}{2\widetilde{R}}\left(\frac{G_-^{(0)}}{\widetilde{R}^2}+\frac{G_+^{(1)}}{c\widetilde{R}}+\frac{G_-^{(2)}}{3c^2}\right) \tag{2}$$

$$B_\theta(\mathbf{r},t) = \frac{A_0\sin\widetilde{\Theta}}{c\widetilde{R}}\left(\frac{G_-^{(1)}}{c\widetilde{R}}+\frac{G_+^{(2)}}{c^2}\right) \tag{3}$$

Where $A_0$ is a parameter related to the amplitude of the field, $\widetilde{R} = [r^2 + (z + \mathrm{i}a)^2]^{1/2}$, $a$ being a parameter related to the beam waist, $\cos\widetilde{\Theta} = (z + \mathrm{i}a)/\widetilde{R}$, $G_\pm^{(n)} = \partial_t^n[f(\widetilde{t}_-) \pm f(\widetilde{t}_+)]$ with $\widetilde{t}_\pm = t \pm \widetilde{R}/c + \mathrm{i}a/c$, $f(t)$ being the inverse Fourier transform of the Poisson-like pulse spectrum $F(\omega)$, given by:

$$F(\omega) = 2\pi\mathrm{e}^{-\mathrm{i}\phi_0}\left(\frac{s}{\omega_0}\right)^{s+1}\frac{\omega^s\mathrm{e}^{-s\frac{\omega}{\omega_0}}}{\Gamma(s+1)}H(\omega) \tag{4}$$

Where $s$ is a parameter related to the duration of the pulse, $\phi_0$ is the absolute phase and $\Gamma$ and $H$ are respectively the gamma and the Heaviside functions. With the notations of the main text, $w_0$ and $\tau_0$ are related to $a$ and $s$ by the following relations: $a = w_0[1 + (1/2k_0w_0)^2]^{1/2}$ [1] and $\omega_0\tau_0 = \sqrt{2}s[4^{1/(s+1)} - 1]^{1/2}$ [2]. The parameters used in the simulations are $k_0a = 70$ and $s = 25$ which correspond to $w_0 = 1.5\,\mu$m and $\tau_0 = 3.5$ fs.

## NUMERICAL PARAMETERS

This section gives details about the numerical parameters of the simulations presented in the main text.

For the plasma mirror simulation, the parameters are the following: space steps $k_0\Delta x = 0.00712$ and $k_0\Delta r = 0.0307$, timestep $\omega_0\Delta t = 0.00601$, 50 electrons per cell, box size $N_z \times N_r = 5624 \times 6552$, 2 orders for the Fourier expansion along the poloidal direction, third order interpolation.

For the gas simulations, the parameters are the following: space steps: $k_0\Delta x = 0.12$ and $k_0\Delta r = 0.4$, timestep $\omega_0\Delta t = 0.1$, 100 atoms per cell with hydrogen, 20 with argon, box size $N_z \times N_r = 3200 \times 360$. 2 orders for the Fourier expansion along the poloidal direction, third order interpolation.

## TRAJECTORIES OF THE FAST ELECTRONS

Figure. S1(a) shows the energy of representative electrons along their trajectories outside the plasma. The electrons are randomly chosen among the electrons with $\theta < 0.1\,\mathrm{rad}$ and $E > 1\,\mathrm{MeV}$. These electrons leave the plasma with an energy of a few hundreds of keV. Most of their final energy is thus gained by VLA in the reflected pulse. Figure. S1(b) shows the work done by the longitudinal field, defined by $WE_z = -e\int \vec{v}.\vec{E_z}dt$, for the same electrons. Figures S1(a) and S1(b) are very similar, proving that electrons are mainly accelerated by the longitudinal electric field of the laser, taking full advantage of the radial polarization. To quantify the impact of the initial velocity given by the plasma, we perform more on-axis test particle simulations. These simulations are performed the same way as the ones shown in Fig. 1 of the main text. The results are shown in Fig. S2. In Fig. S2(a), the electron is initially inside the laser pulse at the optimal initial phase, with no initial velocity. This is the same simulation as in Fig. 1(d) of the main text. In Fig. S2(b), the electron starts at the same position but with an initial velocity of 200 keV in the direction of propagation of the laser, a value corresponding to that observed in the PIC simulation. Adding the initial velocity results in an increase in the energy gain of one order of magnitude (10.2 MeV compared to 1.3 MeV). This shows that the initial velocity given by the plasma capacitor is crucial for our accelerating scheme. Furthermore, the trajectory of the electron in Fig. S2(b) closely resembles that of the fastest electrons in the PIC simulation in Fig. S1(a). This confirms that the longitudinal field $E_z$ is the main driver of the acceleration of the electrons in vacuum.

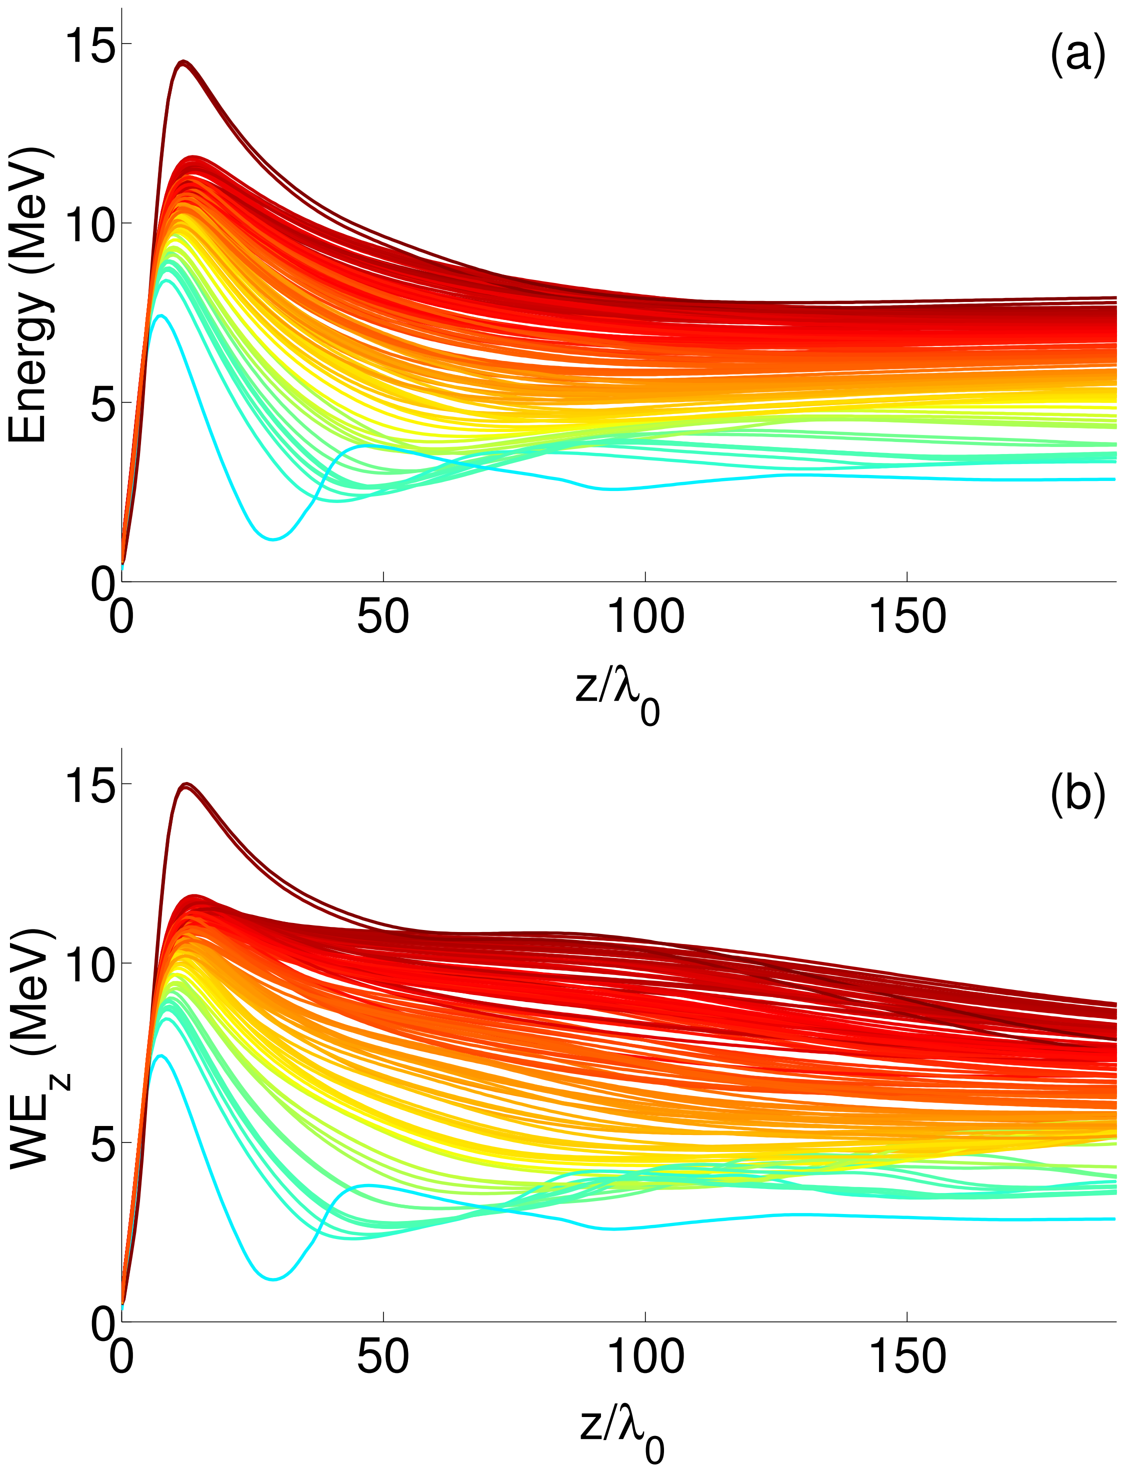


FIG. S1: (a) Energy of some ejected electrons as a function of their distance z from the plasma. (b) Work done by the longitudinal electric field as a function of the distance from the plasma, for these same electrons. The color of the different plots is given by the final energy of the electrons.

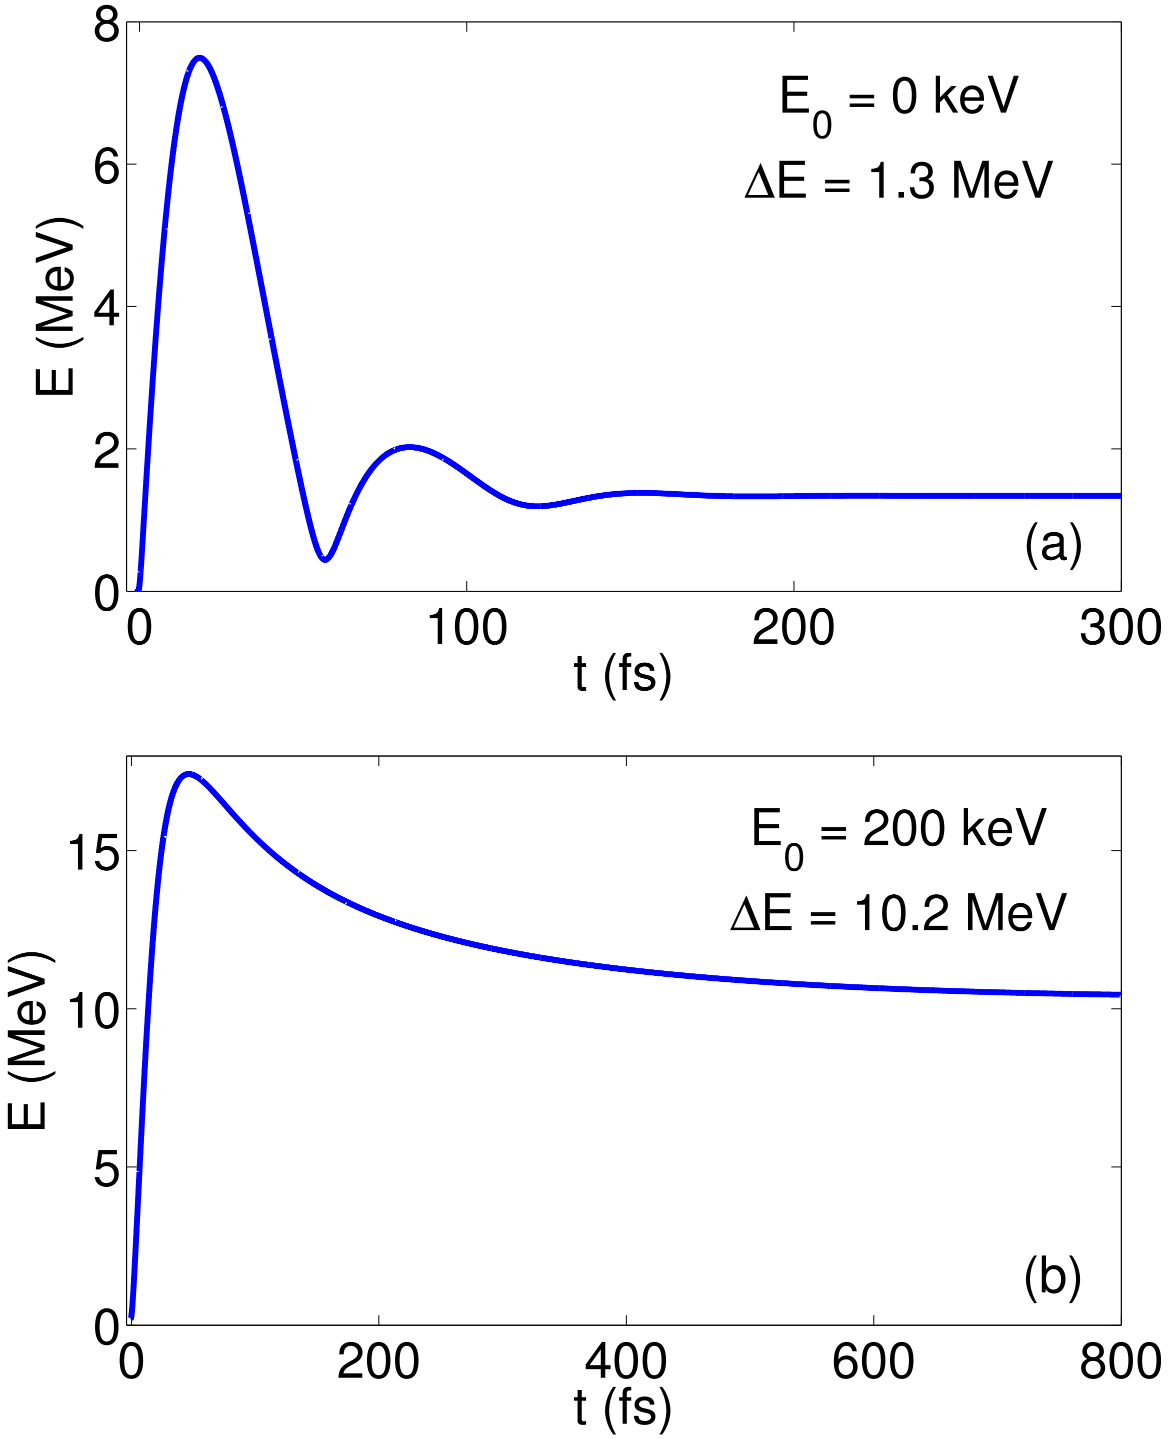


FIG. S2: Result from test particle simulations. Energy of single electrons along their trajectories. The electrons are initially inside the laser pulse at a zero of the longitudinal electric field with either (a) no initial velocity or (b) an initial velocity of 200 keV in the direction of propagation of the laser.

[1] A. April, *Coherence and Ultrashort Pulse Laser Emission* (InTech, 2010), pp. 355–382, F. J. Duarte (ed.).

[2] C. F. R. Caron and R. M. Potvliege, Journal of Modern Optics **46**, 1881 (1999).
